# Supplementary material for: Synthetic non-Abelian gauge fields for non-Hermitian systems
Source: arXiv:2304.01876 ancillary file (2023-04-04)
Supplement: Supplementary file 1 [file SM.pdf]

# Supplementary Materials
# Synthetic non-Abelian gauge fields for non-Hermitian systems

Zehai Pang,[1] Jinbing Hu,[1,2] and Yi Yang[1,*]
[1] Department of Physics, The University of Hong Kong, Pokfulam, Hong Kong, China
[2] College of Optical-Electrical Information and Computer Engineering, University of Shanghai for Science and Technology, Shanghai 200093, China

## S1. HOPF LINK

To characterize the bulk properties of the non-Abelian Hatano–Nelson model, we use the braid degree of a two-strand braid defined by [S1]

$$\nu \equiv \int_0^{2\pi} \frac{\mathrm{d}k}{2\pi \mathrm{i}} \frac{\mathrm{d}}{\mathrm{d}k} \ln \det \left( \hat{H}_k - \frac{1}{2} \mathrm{Tr} \hat{H}_k \right). \tag{S1}$$

Where $\hat{H}_k$ is the Bloch Hamiltonian. The braid degree indicates how many times the two energy bands braid in the $E-k$ space, and the sign shows the handedness of the braid. The absolute value of the braid degree of the non-Abelian Hatano–Nelson model is 2, which indicates that the two energy bands form a Hopf link [S1]. Fig. S1 illustrates the $\nu = \pm 2$ Hopf links (Fig. S1a-b and e-f) and their phase transition under the exceptional-point condition (Fig. S1c-d), and the corresponding projections on the complex energy plane.

## S2. NON-BLOCH WAVE APPROACH

We leverage the non-Bloch approach [S2; S3; S4] to study the non-Hermitian skin effect of both the Abelian and non-Abelian Hatano–Nelson model. In the non-Bloch approach for the one-dimensional (1D) open chain, the Bloch Hamiltonian $H(k)$ can be written as $H(z)$, where $z := \mathrm{e}^{\mathrm{i}k}$, $k \in \mathbb{C}$. The eigenvalue equation $\det[H(z) - E] = 0$ is an algebraic equation for $z$. If the degree of the equation is $2M$, then, the solutions $z_i$ $(i = 1, ..., 2M)$ can be ordered by the absolute value $|z_1| \le |z_2| \le ... \le |z_{2M-1}| \le |z_{2M}|$. The generalised Brillouin zone (GBZ) $C_z$ is given by the trajectory of $z_M$ and $z_{M+1}$ under a condition $|z_M| = |z_{M+1}|$. For each eigen-energy under the open-boundary condition (OBC), there is a corresponding $z_M$, and $|z_M|$ determines the localization of the eigenstate [S4]. If $|z_M| > 1 (< 1)$, the state is right (left) localized. If $|z_M| = 1$, the state is extended.

### A. Lack of tunability with U(1) Abelian gauge fields

Using the non-Bloch approach described above, we can prove that U(1) Abelian gauge fields cannot change the localization of skin modes. The 1D non-Bloch $H_0(z)$ is given by

$$H_0(z) = J_\mathrm{R} \mathrm{e}^{\mathrm{i}\theta_\mathrm{R}} z^{-1} + J_\mathrm{L} \mathrm{e}^{\mathrm{i}\theta_\mathrm{L}} z. \tag{S2}$$

We denote $z_1$ and $z_2$ as solutions to Eq. (S2), which implies

$$\frac{J_\mathrm{R} \mathrm{e}^{\mathrm{i}\theta_\mathrm{R}}}{J_\mathrm{L} \mathrm{e}^{\mathrm{i}\theta_\mathrm{L}}} = z_1 z_2. \tag{S3}$$

The open boundary condition requires

$$|z_1| = |z_2| \tag{S4}$$

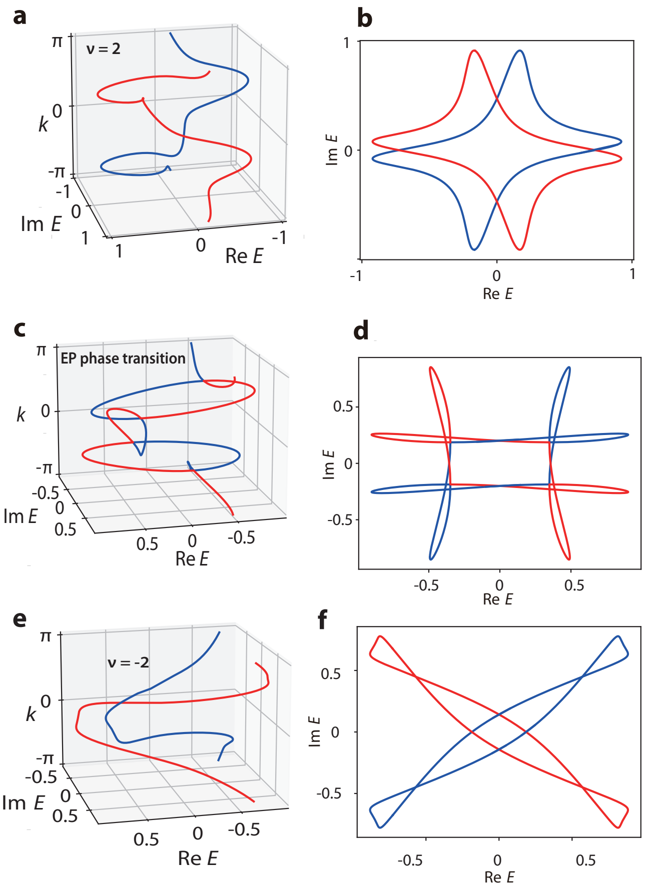


**Figure S1**. **Hopf links formed by energy bands in the** (Re $E$, Im $E$, $k$) **space and their corresponding projections in the complex plane.** Here we use $J_{\mathrm{L}} = 0.7$, $J_{\mathrm{R}} = 0.6$, and $\theta_{\mathrm{R}} = -1.38$ throughout; $\theta_{\mathrm{L}} = -1.5$ for a and b, $\theta_{\mathrm{L}} = -1$ for c and d, and $\theta_{\mathrm{L}} = -0.5$ for e and f respectively. **a,c,e** Braiding of the two bands in (Re $E$, Im $E$, $k$) space. **b,d,f** The corresponding projected energy band in the complex energy plane.

Combining Eqs. (S3) and (S4) yields

$$|z_1| = |z_2| = |J_{\mathrm{R}}/J_{\mathrm{L}}|, \tag{S5}$$

which means that the localization of eigenstates only depends on $|J_{\mathrm{R}}/J_{\mathrm{L}}|$ and the U(1) gauge field cannot modify the localization.

### B. Zero modes of the non-Abelian Hatano–Nelson model

Next, for the non-Abelian Hatano–Nelson model, we prove the existence of the double-degenerate zero modes under OBC. Furthermore, we show that although the skin modes can be effectively tuned by the non-Abelian gauge fields, the localization of the zero modes is solely determined by the imbalance of the hopping amplitudes $J_{\mathrm{L}}$ and $J_{\mathrm{R}}$.

Using the non-Bloch approach, we replace $\mathrm{e}^{\mathrm{i}k}$ with a complex variable $z$ and solve the characteristic polynomial

$$\det[H(z) - E] = J_{\mathrm{L}}^2 z^2 + J_{\mathrm{R}}^2 z^{-2} + 2J_{\mathrm{L}}J_{\mathrm{R}}\cos\theta_{\mathrm{L}}\cos\theta_{\mathrm{R}} - 2E(J_{\mathrm{L}}\cos\theta_{\mathrm{L}} z + J_{\mathrm{R}}\cos\theta_{\mathrm{R}} z^{-1}) + E^2 = 0. \tag{S6}$$

For zero modes $E = 0$, the characteristic polynomial reduces to

$$J_{\mathrm{L}}^2 z^2 + J_{\mathrm{R}}^2 z^{-2} + 2J_{\mathrm{L}}J_{\mathrm{R}}\cos(\theta_{\mathrm{L}})\cos(\theta_{\mathrm{R}}) = 0. \tag{S7}$$

Its four solutions are given by

$$z = \pm \mathrm{i}\sqrt{\frac{J_{\mathrm{R}}}{J_{\mathrm{L}}}(F \pm \mathrm{i}\sqrt{1-F^2})}, \tag{S8}$$

where

$$F = \cos(\theta_{\mathrm{R}})\cos(\theta_{\mathrm{L}}). \tag{S9}$$

The solution $z$ can be re-written as

$$z = \pm \mathrm{i}\sqrt{\frac{J_{\mathrm{R}}}{J_{\mathrm{L}}}}\mathrm{e}^{\pm \mathrm{i}\alpha}, \tag{S10}$$

where

$$\alpha = \arctan(\frac{\sqrt{1-F^2}}{F}). \tag{S11}$$

Eq. (S10) shows that all four roots have the same absolute value, meaning that the zero modes always exist under OBC. Furthermore, the roots are independent of the Abelian gauge fields, which implies the localization of the zero modes only depends on the hopping amplitudes. Since all four solutions have the same absolute value, it is free to choose $z_2$ and $z_3$ to plot the GBZ. Moreover, the connectivity and closure requirement of GBZ [S5] requires that all four roots must appear on the GBZ, which enforces that the zero modes must be doubly degenerate and that each mode contributes to a pair of roots to the GBZ.

## S3. WINDING-NUMBER APPROACH

Recently, the correspondence between the winding number under the periodic boundary condition (PBC) and the OBC skin effect has been rigorously established for 1D single-band systems [S5]. Such correspondence can be extended into multi-band systems as long as the winding number of each band can be well-defined, which holds for the non-Abelian Hatano–Nelson model.

For a 1D non-Hermitian lattice system, the OBC spectrum is always encircled by the PBC spectrum [S6]. Therefore, for each OBC energy base point $E_{\mathrm{b}}$, a multi-band topological winding number $w$ can be defined as [S7]

$$w(E_{\mathrm{b}}) \equiv \sum_{n=1}^{N}\int_{-\pi}^{\pi}\frac{\mathrm{d}k}{2\pi}\partial_k \arg\left[(E_n(k)-E_{\mathrm{b}}\right], \tag{S12}$$

where $n$ indicates the index of the energy band, $N$ is the total number of bands, and $\arg E_n(k)$ is the argument of complex energy band $E_n(k)$. The sign of $w$ indicates the localization of skin modes, i.e. a positive and negative $w$ indicates left- and right-localization, respectively.

From the winding-number approach, it is also possible to discuss the properties of zero-mode localization. If we choose zero energy as the base energy point, a phase transition requires that $w(0)$ should change sign. The phase transition point is given by $\det H(k) = 0$, which requires simultaneously

$$\begin{cases} J_{\mathrm{L}}^2\cos 2k + J_{\mathrm{R}}^2\cos 2k + 2J_{\mathrm{L}}J_{\mathrm{R}}\cos\theta_{\mathrm{R}}\cos\theta_{\mathrm{L}} = 0, & \text{(S13a)} \\ J_{\mathrm{L}}^2\sin 2k - J_{\mathrm{R}}^2\sin 2k = 0 & \text{(S13b)} \end{cases}$$

When $|J_{\mathrm{L}}| \neq |J_{\mathrm{R}}|$, Eq. (S13b) requires $\sin 2k = 0$ and thus $\cos 2k = \pm 1$, which combines with Eq. (S13a) yielding

$$\pm\frac{J_{\mathrm{L}}^2 + J_{\mathrm{R}}^2}{2J_{\mathrm{L}}J_{\mathrm{R}}} = \cos\theta_{\mathrm{R}}\cos\theta_{\mathrm{L}}. \tag{S14}$$

Eq. (S14) is impossible because $J_{\mathrm{L}}^2 + J_{\mathrm{R}}^2 > 2J_{\mathrm{L}}J_{\mathrm{R}}$ for $|J_{\mathrm{L}}| \neq |J_{\mathrm{R}}|$,. As a result, the zero-energy phase transition is not possible when $|J_{\mathrm{L}}| \neq |J_{\mathrm{R}}|$.

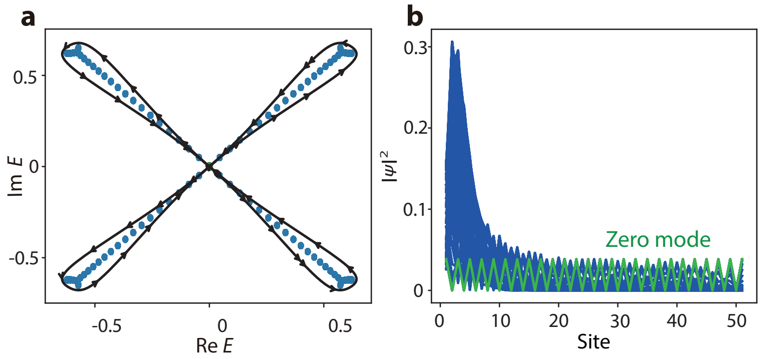


**Figure S2**. **zero-energy phase transition. a.** PBC and OBC energy spectra in the complex plane. **b.** All modes are left-localized except the zero modes (green color) that are extended. $|J_L| = |J_R| = 0.5$, $\theta_R = 2.7$, $\theta_L = 1.5$. The chain length is 50.

Alternatively, for $|J_L| = |J_R|$, the zero-energy phase transition requires

$$\cos 2k = -\cos\theta_L \cos\theta_R, \tag{S15}$$

which can be always be met for a certain $k \in [-\pi, \pi]$.

Therefore, $|J_L| = |J_R|$ corresponds to the only zero-energy phase transition, which does not involve $\theta_L$ and $\theta_R$. In other words, $\theta_L$ and $\theta_R$ cannot change zero modes' winding number and their localization. Also, based on the previous section, we know that zero modes always exist, and they are doubly degenerate with the same localization. Thus, the two PBC energy bands surrounding the zero energy must share the same orientation. The existence of zero modes also indicates that the two PBC energy bands are point-gaped with base energy zero since zero energy can never be placed outside of the PBC energy bands. A typical spectrum and its skin modes are given in Fig. S2 for $|J_L| = |J_R|$, which numerically show a zero-energy phase transition and the same orientation of the two PBC bands.

## S4. ASYMPTOTIC ANALYSIS

To understand the role of non-Abelian gauge fields, we studied the asymptotic behavior of the energy band. By performing Taylor expansion, we found that the effective high-order hopping and nearest-neighbor hopping are comparable near the exceptional condition to the first-order approximation. As a result, the tuning mechanism is the result of the competition between nearest-neighbor hopping and effective high-order hopping.

We can rewrite the eigen-energy of the non-Abelian Hatano–Nelson model

$$E_\pm(k) = A(k) \pm \mathrm{i}\sqrt{J_L^2 \sin^2\theta_L \mathrm{e}^{\mathrm{i}2k} + J_R^2 \sin^2\theta_R \mathrm{e}^{-\mathrm{i}2k}}, \tag{S16}$$

where

$$A(k) = J_L \cos\theta_L \mathrm{e}^{\mathrm{i}k} + J_R \cos\theta_R \mathrm{e}^{-\mathrm{i}k}. \tag{S17}$$

Without loss of generality, we assume $|J_L| > |J_R|$. To study the asymptotic behaviour, we can first assume $(\frac{J_R \sin\theta_R}{J_L \sin\theta_L})^2 < 1$, and Eq. (S16) can be reformulated as

$$E_\pm(k) = A(k) \pm \mathrm{i}J_L \sin\theta_L \mathrm{e}^{\mathrm{i}k}\sqrt{1 + (\frac{J_R \sin\theta_R}{J_L \sin\theta_L})^2 \mathrm{e}^{-\mathrm{i}4k}}, \tag{S18}$$

which permits a Taylor expansion in the form of

$$E_\pm(k) = A(k) \pm \mathrm{i}J_L \sin\theta_L e^{ik}\left[1 + \frac{1}{2}\left(\frac{J_R \sin\theta_R}{J_L \sin\theta_L}\right)^2 \mathrm{e}^{-\mathrm{i}4k} - \frac{1}{8}\left(\frac{J_R \sin\theta_R}{J_L \sin\theta_L}\right)^4 \mathrm{e}^{-\mathrm{i}8k} + \cdots\right]. \tag{S19}$$

The first term in the bracket is a Hatano–Nelson term that does not modify the non-hermitian skin effect (NHSE). When $(\frac{J_R \sin\theta_R}{J_L \sin\theta_L})^2 \ll 1$, to first-order approximation the Hatano–Nelson term is dominated. Then Eq. (S19) can be approximated as $E_\pm(k) \simeq J_L e^{\pm i\theta_L} e^{ik} + J_R \cos\theta_R e^{-ik}$. Since $|J_L e^{\pm i\theta_L}| > |J_R \cos\theta_R|$, all states are left-localized when $(\frac{J_R \sin\theta_R}{J_L \sin\theta_L})^2 \ll 1$.

Similarly, when $(\frac{J_R \sin\theta_R}{J_L \sin\theta_L})^2 > 1$, we can rewrite Eq. (S16) as

$$E_\pm(k) = A(k) \pm iJ_R \sin\theta_R e^{-ik}\left[1 + \frac{1}{2}\left(\frac{J_L \sin\theta_L}{J_R \sin\theta_R}\right)^2 e^{i4k} - \frac{1}{8}\left(\frac{J_L \sin\theta_L}{J_R \sin\theta_R}\right)^4 e^{i8k} + \cdots\right]. \tag{S20}$$

If $(\frac{J_R \sin\theta_R}{J_L \sin\theta_L})^2 \gg 1$, Eq. (S20) can be approximated as $E_\pm(k) \simeq J_L \cos\theta_L e^{ik} + J_R e^{\pm i\theta_R} e^{-ik}$. Thus, it additionally requires $|J_L \cos\theta_L| \geq |J_R e^{\pm i\theta_R}| = |J_R|$ such that all states are left-localized.

When $(\frac{J_R \sin\theta_R}{J_L \sin\theta_L})^2 \approx 1$, i.e. near the exceptional-point condition, higher-order terms becomes non-negligible in both Eqs. (S19) and (S20). Taken together, near the exceptional-point condition and in the vicinity of the $(\theta_L, \theta_R)$ parameter space complementary to $|J_L \cos\theta_L| \geq |J_R| \cup (\frac{J_R \sin\theta_R}{J_L \sin\theta_L})^2 \ll 1$, non-Abelian gauge fields enable the simultaneous presence of NHSE on both ends of the open chain and their localization tunability.

## REFERENCES

* yiyg@hku.hk

[S1] K. Wang, A. Dutt, C. C. Wojcik, and S. Fan, Nature **598**, 59 (2021).
[S2] S. Yao and Z. Wang, Physical review letters **121**, 086803 (2018).
[S3] Z. Yang, K. Zhang, C. Fang, and J. Hu, Physical Review Letters **125**, 226402 (2020).
[S4] K. Yokomizo and S. Murakami, Physical review letters **123**, 066404 (2019).
[S5] K. Zhang, Z. Yang, and C. Fang, Physical Review Letters **125**, 126402 (2020).
[S6] Y. Ashida, Z. Gong, and M. Ueda, Advances in Physics **69**, 249 (2020).
[S7] Z. Gong, Y. Ashida, K. Kawabata, K. Takasan, S. Higashikawa, and M. Ueda, Physical Review X **8**, 031079 (2018).
